# Supplementary material for: Multi-Objective Model-based Reinforcement Learning for Infectious Disease Control
Source: arXiv:2009.04607 source file (2022-02-26)
Supplement: Supplementary file 3 [file appendix_posterior.tex]

\section{Posterior estimation of the GSIR model}\label{sec:MAP}
In this section, we introduce the derivation of the posteriors. 
% our prior family choices for $\vthe$ and
Recall our model (\ref{SIR}) is 
\begin{align*}
% \begin{split}
X^S_{l,t+1} &= X^S_{l,t} - e^S_{l,t}, e^S_{l,t} \sim  \text{Poisson}(\sum_{j=1}^J \beta_j \mathbb{I}(A_{l,t} = j) X^S_{l,t} \frac{X^I_{l,t}}{M_l}) ;\\ %   \hl{notation?}
X^R_{l,t+1 } &= X^R_{l,t} + e^R_{l,t}, e^R_{l,t} \sim \text{Binomial}(X^I_{l,t}, \gamma );\\
X^I_{l,t+1} &= M_l - X^S_{l,t+1} - X^R_{l,t+1 }, 
% \end{split}
\end{align*}
where the third equation is redundant. 
With data $\mathcal{D}_{t_0}$, the Markov property of the transition model reduces the estimation problem to $J + 1$ Bayesian generalized linear models with the identity link function. 
Specifically, let ${\Omega_{t_0,j}} = 
\{(t,l): 1 \leq t \leq t_0 - 1,
1 \leq l \leq N_{t}, 
A_{l,t} = j\}$ be the set of time-location pairs where action $j$ is taken, and let $\Omega_{t_0} = \{(t,l): 1 \leq t \leq t_0 - 1,
1 \leq l \leq N_{t}\}$. 
Assume $\{e^S_{l.t}, e^R_{l.t}|  1 \leq t \leq t_0 - 1,
1 \leq l \leq N_{t} \}$ are all independent, and then the likelihood function can be written as 
\begin{align*}
&\mathcal{L}( \vthe |\mathcal{D}_{t_0}) 
= \prod_{(t,l) \in \Omega_{t_0}} f_B(X^R_{l,t+1 } - X^R_{l,t}, X^I_{l,t}; \gamma)  \\
&\quad \times \prod_{j \in \{1, \dots, J\} } \prod_{(t,l) \in \Omega_{t_0,j}} f_P(
X^S_{l,t} - X^S_{l,t+1}; %\\ 
\sum_{j=1}^J \beta_j \mathbb{I}(A_{l,t} = j)  X^S_{l,t} X^I_{l,t} / M_l ), 
\end{align*} 
where $f_B(\cdot, \cdot; \cdot)$  is the density function of the Binomial distribution and $f_P(\cdot; \cdot)$ is that of the Poisson distribution. 
For simplicity, we consider the case that the parameter priors are independent with each other. 
For more general settings, approximate inference methods such as Markov Chain Monte Carlo can be used. 
For the recover rate $\gamma$, we use the Beta-Binomial conjugate pair and set its prior as $Beta(a_{R}, b_{R})$ with parameters 
$a_{R}$ and  $b_{R}$. 
For the infection rate $\beta_j$, $j = 1, \dots, J$, the Poisson-Gamma conjugate pair is used,
and we set the prior of $\beta_j$ as $ Beta(a_{S,j}, b_{S,j})$ with parameters 
$a_{S, j}$ and  $b_{S, j}$. 
By choosing these conjugate priors, the corresponding posterior distributions have explicit forms as $\gamma \mid \mathcal{D}_{t_0} \sim  Beta(a_{R}^* , b_{R}^*)$ 
and 
$\beta_j \mid \mathcal{D}_{t_0} \sim  Gamma(a_{S,j}^* , b_{S,j}^*)$, for $j = 1, \dots, J$
, where

\begin{equation*}
    \begin{aligned}
a_{S,j}^* &= a_{S,j} + \sum_{(t,l) \in \Omega_{t_0,j}}\left( {X_{l, t}^{S} - X_{l, t+1}^{S}}{} \right),\\
b_{S,j}^* &= b_{S,j}+ \sum_{(t,l) \in \Omega_{t_0,j}}  \frac{X_{l, t}^{S,j}X_{l, t+1}^{I}}{M_l}, \\
a_{R}^* &= a_{R} + \sum_{(t,l) \in \Omega_{t_0}} \left( {X_{l, t+1}^{R} - X_{l, t}^{R}} \right), \\ % (t,l)  because l \leq N_t depends on t --> t first then l or (l, t) location \sum_{l=1}^{N_{t_0}} \sum_{t=t_l}^{t_0-1}, where $t_l$ is the first day when region l has confirmed cases.
b_{R}^* &= b_{R}- \sum_{(t,l) \in \Omega_{t_0}}  \left( {X_{l, t+1}^{R} - X_{l, t}^{R}} \right) + \sum_{(t,l) \in \Omega_{t_0}} {X_{l, t}^{I}}.
\end{aligned}
\end{equation*}
\raggedbottom



%%%%%%%%%%%%%%%%%%%%%%%%%%%%%%%%%%%%%%%%
%%%%%%%%%%%%%%%%%%%%%%%%%%%%%%%%%%%%%%%%
