# Supplementary material for: Multi-Objective Model-based Reinforcement Learning for Infectious Disease Control
Source: arXiv:2009.04607 source file (2022-02-26)
Supplement: Supplementary file 4 [file suppCOVID.tex]

% \usepackage{amssymb}
\input{0_KDD_pre}
\usepackage{subcaption}

\usepackage{xr}
\makeatletter

\newcommand*{\addFileDependency}[1]{% argument=file name and extension
  \typeout{(#1)}
  \@addtofilelist{#1}
  \IfFileExists{#1}{}{\typeout{No file #1.}}
}
\makeatother

\newcommand*{\myexternaldocument}[1]{%
    \externaldocument{#1}%
    \addFileDependency{#1.tex}%
    \addFileDependency{#1.aux}%
}

\myexternaldocument{./0_MAIN}



\title{Supplement to ``Multi-Objective Model-based Reinforcement Learning for Infectious Disease Control"}

\begin{document}
\setcounter{section}{1}
	
\maketitle

\appendix 



\raggedbottom
\section{Posterior estimation of the GSIR model}\label{sec:MAP}
In this section, we introduce the derivation of the posteriors. 
% our prior family choices for $\vthe$ and
Recall our model (\ref{SIR}) is 
\begin{align*}
% \begin{split}
X^S_{l,t+1} &= X^S_{l,t} - e^S_{l,t}, e^S_{l,t} \sim  \text{Poisson}(\sum_{j=1}^J \beta_j \mathbb{I}(A_{l,t} = j) X^S_{l,t} \frac{X^I_{l,t}}{M_l}) ;\\ %   \hl{notation?}
X^R_{l,t+1 } &= X^R_{l,t} + e^R_{l,t}, e^R_{l,t} \sim \text{Binomial}(X^I_{l,t}, \gamma );\\
X^I_{l,t+1} &= M_l - X^S_{l,t+1} - X^R_{l,t+1 }, 
% \end{split}
\end{align*}
where the third equation is redundant. 
With data $\mathcal{D}_{t_0}$, the Markov property of the transition model reduces the estimation problem to $J + 1$ Bayesian generalized linear models with the identity link function. 
Specifically, let ${\Omega_{t_0,j}} = 
\{(t,l): 1 \leq t \leq t_0 - 1,
1 \leq l \leq N_{t}, 
A_{l,t} = j\}$ be the set of time-location pairs where action $j$ is taken, and let $\Omega_{t_0} = \{(t,l): 1 \leq t \leq t_0 - 1,
1 \leq l \leq N_{t}\}$. 
Assume $\{e^S_{l.t}, e^R_{l.t}|  1 \leq t \leq t_0 - 1,
1 \leq l \leq N_{t} \}$ are all independent, and then the likelihood function can be written as 
\begin{align*}
&\mathcal{L}( \vthe |\mathcal{D}_{t_0}) 
= \prod_{(t,l) \in \Omega_{t_0}} f_B(X^R_{l,t+1 } - X^R_{l,t}, X^I_{l,t}; \gamma)  \\
&\quad \times \prod_{j \in \{1, \dots, J\} } \prod_{(t,l) \in \Omega_{t_0,j}} f_P(
X^S_{l,t} - X^S_{l,t+1}; %\\ 
\sum_{j=1}^J \beta_j \mathbb{I}(A_{l,t} = j)  X^S_{l,t} X^I_{l,t} / M_l ), 
\end{align*} 
where $f_B(\cdot, \cdot; \cdot)$  is the density function of the Binomial distribution and $f_P(\cdot; \cdot)$ is that of the Poisson distribution. 
For simplicity, we consider the case that the parameter priors are independent with each other. 
For more general settings, approximate inference methods such as Markov Chain Monte Carlo can be used. 
For the recover rate $\gamma$, we use the Beta-Binomial conjugate pair and set its prior as $Beta(a_{R}, b_{R})$ with parameters 
$a_{R}$ and  $b_{R}$. 
For the infection rate $\beta_j$, $j = 1, \dots, J$, the Poisson-Gamma conjugate pair is used,
and we set the prior of $\beta_j$ as $ Beta(a_{S,j}, b_{S,j})$ with parameters 
$a_{S, j}$ and  $b_{S, j}$. 
By choosing these conjugate priors, the corresponding posterior distributions have explicit forms as $\gamma \mid \mathcal{D}_{t_0} \sim  Beta(a_{R}^* , b_{R}^*)$ 
and 
$\beta_j \mid \mathcal{D}_{t_0} \sim  Gamma(a_{S,j}^* , b_{S,j}^*)$, for $j = 1, \dots, J$
, where

\begin{equation*}
    \begin{aligned}
a_{S,j}^* &= a_{S,j} + \sum_{(t,l) \in \Omega_{t_0,j}}\left( {X_{l, t}^{S} - X_{l, t+1}^{S}}{} \right),\\
b_{S,j}^* &= b_{S,j}+ \sum_{(t,l) \in \Omega_{t_0,j}}  \frac{X_{l, t}^{S,j}X_{l, t+1}^{I}}{M_l}, \\
a_{R}^* &= a_{R} + \sum_{(t,l) \in \Omega_{t_0}} \left( {X_{l, t+1}^{R} - X_{l, t}^{R}} \right), \\ % (t,l)  because l \leq N_t depends on t --> t first then l or (l, t) location \sum_{l=1}^{N_{t_0}} \sum_{t=t_l}^{t_0-1}, where $t_l$ is the first day when region l has confirmed cases.
b_{R}^* &= b_{R}- \sum_{(t,l) \in \Omega_{t_0}}  \left( {X_{l, t+1}^{R} - X_{l, t}^{R}} \right) + \sum_{(t,l) \in \Omega_{t_0}} {X_{l, t}^{I}}.
\end{aligned}
\end{equation*}
\raggedbottom



%%%%%%%%%%%%%%%%%%%%%%%%%%%%%%%%%%%%%%%%
%%%%%%%%%%%%%%%%%%%%%%%%%%%%%%%%%%%%%%%%

\section{More on the Policy Search Algorithms}
\subsection{Constrained simultaneous perturbation stochastic approximation}\label{sec:SPSA}

When $J$ is large, Algorithm \ref{alg:grid} in the main paper can be computationally expensive. 
In general, a variety of optimization algorithms, such as Bayesian optimization and heuristic optimization algorithms, can be applied here. 
As an example, we provide a constrained simultaneous perturbation stochastic approximation (SPSA) algorithm  \cite{sadegh1997constrained} here. 
%  for more general settings
It is described in Algorithm \ref{alg:SPSA}. 
In SPSA, we need to specify two step size sequences $\{\zeta_k\}_{k\ge 1}$ and $\{\xi_k\}_{k\ge 1}$, which  should satisfy $\sum_{k = 1}^{\infty} \zeta_k = \infty, \sum_{k = 1}^{\infty} \zeta_k^2 < \infty$ and $\xi_k = o(1)$ as $k$ goes to infinity. %? not uniform?
% In our experiments, we use $\zeta_k = \zeta / k^{\tau}$ and $\xi_k = \xi/k$, where $\zeta, \xi$  and $\tau \in (0.5,1]$ are  tuning parameters. 
Unlike traditional SPSA, for each candidate parameter $\vlam_t^k$, we run $M$ replications of Monte Carlo instead of only once and use the average to approximate the expected average utility. 
This is because that, in our setting, the sampling is relatively cheap and the potential loss of a sub-optimal policy can be quite severe. 
The operator $\mathbb{P}_{E_k}$ is the orthogonal projection onto  $E_k$ and it ensures the feasibility of policy evaluation under the constraints. 
Following \cite{sadegh1997constrained}, we define $E_k = \{\vlam: \lam_J + \xi_k\sqrt{J - 1} \le \lam_M, \lam_i + \xi_k\sqrt{J - 1} \le \lam_{i + 1} , \forall i \in \{1,\dots,J-1\} \}$. 
The direction is sampled from a distribution $\mathbb{G}$ of dimension $J-2$. 
The convergence of SPSA is guaranteed by our choice of $\zeta_k$.
In implementations, 
warm start can be used by setting $\vlam^1 = \vlam_{t_0 - 1}$ to further reduce the computational burden and 
multi-start random initialization can also be employed to remedy the non-convexity. 
% \hl{needs update Ek. already done in the code}
% Denote the feasible parameter region as $E = \{\vlam: 0 \le \lam_2 \le \dots \le \lam_{J} \le \lam_M\}$. 


\input{Algorithms/Algo_SPSA.tex}


\subsection{Deep Q-learning}\label{sec:supp-DQN}
When the global optimality is preferred, we can choose a general policy class and apply cutting-edge RL algorithms to solve the planning problem. 
In Algorithm \ref{alg:DQN}, we modify the deep-Q learning algorithm to take into consideration the learned uncertainty on $\vthe$.  
% used in our experiment. 
More details abou the standard DQN can be found in \cite{mnih2015human}. 


\input{Algorithms/DQN}




\subsection{Computational complexity}\label{sec:complexity}

In this section, we discuss the computational complexity of our policy search algorithm. 
We first consider a general form of the grid search algorithm presented in Algorithm \ref{alg:grid}. 
Suppose we have $J$ action levels, and recall we have $J - 1$ policy parameters $\lam_2, \dots, \lam_J$. 
Let the step size for searching $\lam_j$ be $\xi_j$ and the corresponding upper search bound be $U_j$, for $j = 2, \dots, J$. 
Define $\eta = max_{j \in \{2, \dots, J\}} (U_j / \xi_j)$. 
Assume that for each candidate policy, we run $M$ replications of rollouts.  
Using similar iteration schedule with Algorithm \ref{alg:grid} in the main paepr,
the computational complexity is easy to calculate as $O(M T \eta^{J - 1})$, where $T$ is the horizon. 
Then it is straightforward to show that the computational complexity of Algorithm 1 is $O(MB T \eta^{J - 1} + BKT)$, where $B$ is the number of candidate weights and $K$ is the number of Monte Carlo replications. 
Due to the importance of a stable optimization algorithm in our application, we choose to use this grid search algorithm in our experiment and recommend a large $M$. 
This is feasible when $J$ is not large, for example, $3$ or $5$. 
However, because its complexity is of exponential order with respect to $J$, when there are many actions available, we should choose other optimization algorithms such as Algorithm \ref{alg:SPSA}, with a large $M$ to reduce the variance from Monte Carlo rollouts. 
The algorithm is embarrassingly parallel. 
For the DQN-based method, the complicity is $B$ times of that of the standard deep-Q learning algorithm. 

\subsection{Hyper-parameters}
In this section, we describe the hyper-parameters used in our experiments. 
For the grid search algorithm, the number of rollout replications is set as $M = 100$. 
We run the grid search algorithm from coarse grids to finer grids to save computational cost. 
The schedule is listed in Table \ref{table:para}. 
In generally, the larger the search spaces and the smaller the step sizes, the better the performance will be. 
In consideration of the importance of this application and the relatively lightweight computation, in real application, we can choose the search spaces as large enough and step size as small enough. 
% $\lambda_M$ is another upper bound which indicates that, no matter

For DQN, in our experiment, we use a dense network of 5 layers, with 32 nodes per layer, to model the Q-function. 
The activation function is picked as relu and the optimizer is set as Adam. 
The learning rate is fixed as 0.0002 and the parameter for epsilon-greedy is set as $\epsilon = 0.1$. 
% max_epoch = 100


% &   $\beta_3$ 
\begin{table*}[t!]
\centering
    \caption{Search space and step sizes for the grid search in each round. $\lam^i_1$ and $\lam^i_2$ are the output from the $i$-th round.}
    \label{table:para}
    \begin{tabular}{lllllll}
\toprule
  round & $u_2$  &  $u_3$    & $U_2$  & 
  $U_3$ &   $\xi_2$ &   $\xi_3$  \\
\midrule
1 & 0& 300& 50& 0& 100& 200 \\
2 &  max(0, $\lam^1_1$ - 50)&  $\lam^1_1$ + 50& 5& $\lam^1_2$ - 200& $\lam^1_2$ + 200& 20 \\
3 &  max(0, $\lam^2_1$ - 5)&  $\lam^2_1$ + 5& 1& $\lam^2_2$ - 20& $\lam^2_2$ + 20& 4 \\
4 &  max(0, $\lam^3_1$ - 1)&  $\lam^3_1$ + 1& 0.25& $\lam^3_2$ - 4& $\lam^3_2$ + 4& 1 \\
5 &  max(0, $\lam^4_1$ - 0.25)&  $\lam^4_1$ + 0.25& 0.01& $\lam^4_2$ - 1& $\lam^4_2$ + 1& 0.2 \\
\bottomrule
\end{tabular}
\end{table*}
%%%%%%%%%%%%%%%%%%%%%%%%%%%%%%%%%%%%%%%%%%%%%%%%
%%%%%%%%%%%%%%%%%%%%%%%%%%%%%%%%%%%%%%%%%%%%%%%%

\section{Details of the numerical experiments}

% In this section, we provide mores details of Section \ref{sec:numerical} and addtional numerical results. 

\subsection{More on the China COVID-19 dataset and hyper-parameters}\label{sec:supp-data}

We obtain the counts of cumulative confirmed cases $O_{l,t}^I$ from  \cite{China_Data} with irregular records imputed by the average of their neighbors.
The original mobility data collected from the online plateform Baidu Qianxi\footnote{http://qianxi.baidu.com} includes ${m_{l,t}^{20}}$, the mobility of people in city $l$ on day $t$ in  2020, and ${m_{l,t}^{19}}$, the value for the same date in 2019, aligned by the lunar calendar.  
We define $r_{l,t}=1- m_{l,t}^{20}/m_{l,t}^{19}$ to 
measure the  ratio of human mobility loss due to $A_{l,t}$. 
The fitted distributions for the intervention cost function are $C_2 \sim \mathcal{N}(0.368, 0.239^2)$ and 
$C_3 \sim \mathcal{N}(0.484, 0.181^2)$.
% C_3 rather than C_2
As for the action data, we collect the date ranges for different control measures claimed by Chinese local governments. 
The date ranges for action $1$ and $2$ as well as the starting dates for action $3$ are collected from \cite{wiki:action}. 
The ending dates for action $3$ are manually collected from the local government websites or their social media accounts. 
These data sources are all in Chinese. 
We use the estimates for SARS \cite{mkhatshwa2010modeling} to set the priors for the disease features, specifically, we set $\gamma \sim Beta(178.89, 2000)$ and $ \beta_1 \sim Gamma(517.41, 2000)$.
As for $\beta_2$ and $\beta_3$, similar with the assumptions in \cite{ferguson2020impact}, we assume the two measures reduce the infection rate by $80\%$ and $90\%$ respectively, and therefore use $\beta_2 \sim Gamma(103.48 , 2000)$ and $ \beta_3 \sim Gamma(51.74, 2000)$. 


% Since $X_{l,t}^R$ should be monotonically non-decreasing with respect to $t$ and there are some records violating this quality, we have substituted the peculiar records with mean values of their neighbors. 
% Figure \ref{fig:cost} shows the boxplot of the mobility loss ratio for different actions. 




\subsection{Validation of the simulation environment}\label{sec:supp_val}

We apply a leave-one-out cross-validation procedure to show that our simulation environment is close to the real data generation process. 
Specifically, for $l = 1, \dots, 6$, we follow the steps: 
\begin{enumerate}
    \item estimate the environmental parameter $\vthe$ as $\hat{\vthe}_l$, using all data  until day $61$ of cities in $\{1, \dots, 6\} \setminus \{l\}$.
    % day 10 = [2020-01-24]
    % day 61 = [2020-03-15]
    % day 120 = [2020-05-13]
    \item for city $l$, based on $\hat{\vthe}_l$, we predict its counts of the cumulative infected cases from day $12$ to day $120$, following the observed actions in the data. Denote the estimate for day $120$ as $\hat{X}^R_{120, l}.$ 
    % , t=10, 11,\cdots, 120$.
    \item calculate the approximation error by $\epsilon_{l} = |\hat{X}^R_{120, l} - O^I_{120,l}| / O^I_{120,l}$, where $O^I_{120,l}$ is the observed cumulative infected count for city $l$ until day $120$. 
\end{enumerate}

The average error ratio $\sum_{l = 1}^6 \epsilon_{l} / 6 = 0.18$  indicates that the environment is a relatively valid proxy for the real data generation process, 
and supports the fairness of our comparison with the behaviour policy. 

\subsection{Statistical significance of the policy evaluation results}

In Figure \ref{figure:Pareto} in the main paper, we compare  our algorithm with the other competing policies by 
the average costs following each policy. 
To examine the statistical significance of our results, we report the corresponding $95\%$ confidence interval for each average value in Figure \ref{figure:Paretosquare}. 
We can observe that our findings in Section \ref{sec:policy} are  statistically significant. 
The variance for the DQN-based method is slightly larger due to the limited computational resources, and we expect it will become stabler with more computation. 
Results for the other experiments are similar. 

% \begin{figure}[h]
% 	\centering
% 	\includegraphics[width=0.9\textwidth]{figures/more_final_val.png}
% 	\caption{Validation result with the least RMSE, where $\mathcal{L}_i=\{$Beijing, Guangzhou, Shanghai$\}$ and $\mathcal{L}'_i=\{$Hefei, Nanjing, Tianjin$\}.$}\label{fig:cv3}
% \end{figure}

\begin{figure}[h!]
\centering
\includegraphics[width=.5\textwidth]{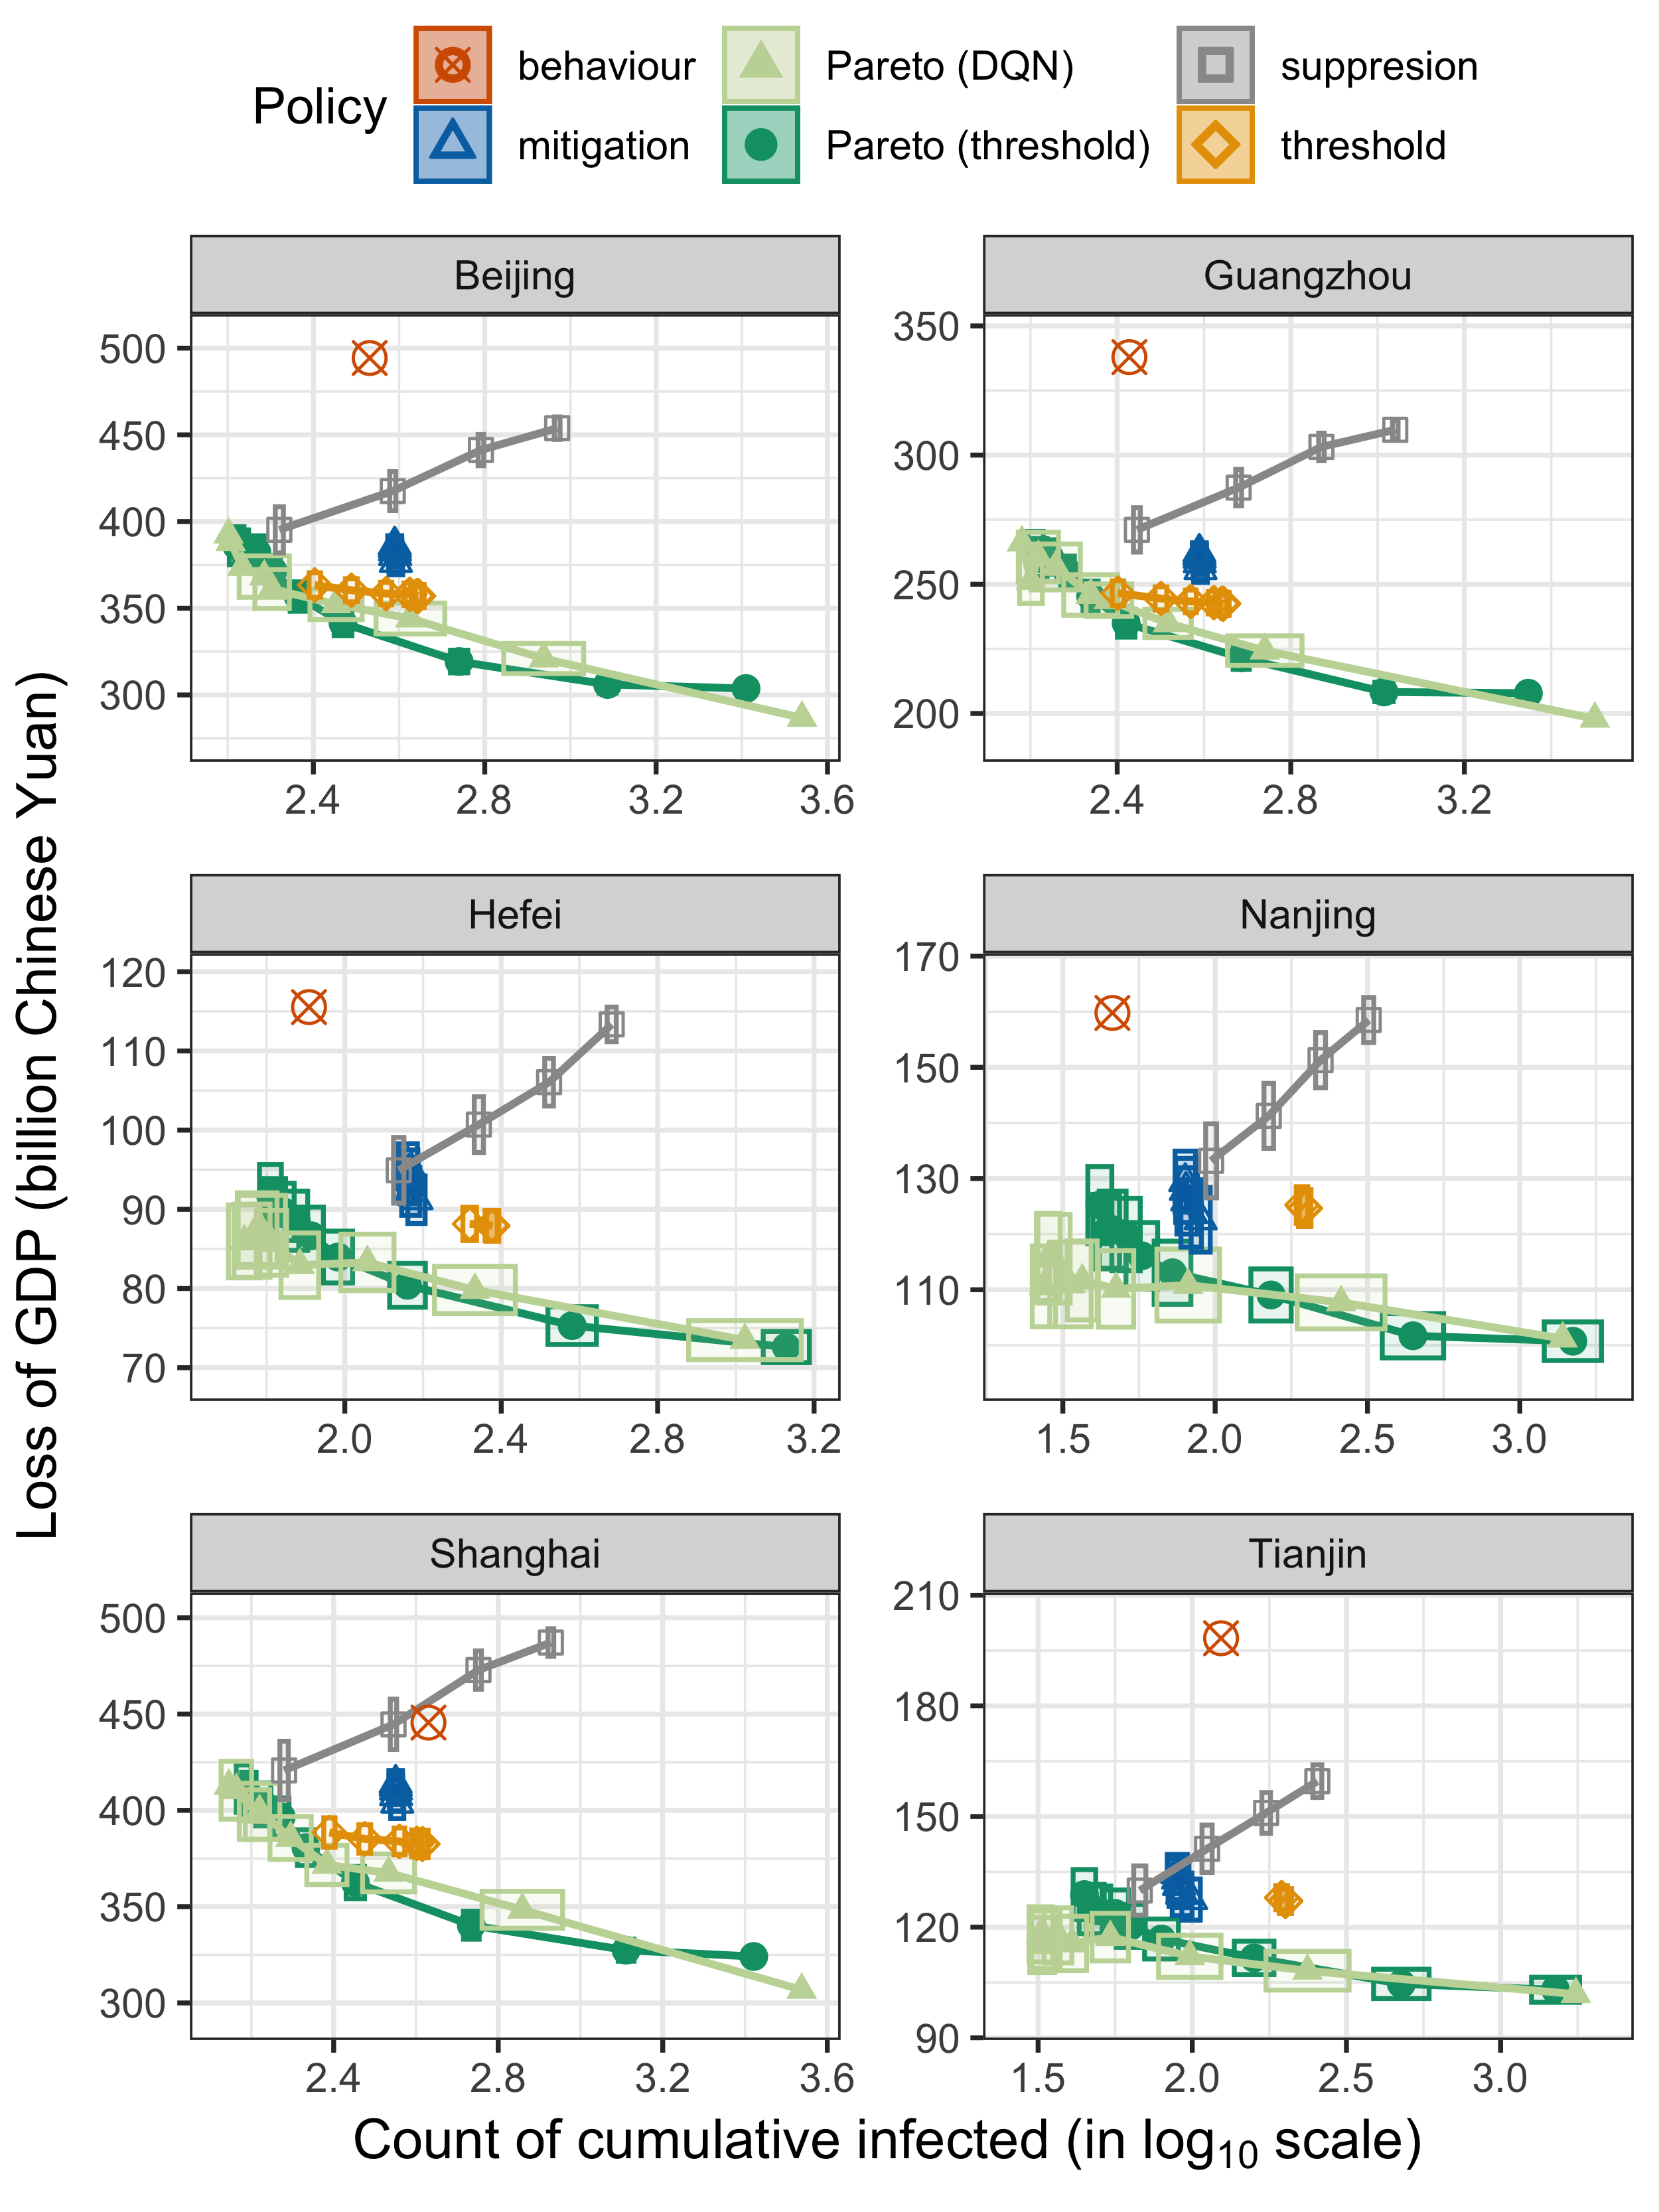} 
% Figure1_supp_factor10
\caption{Cumulative epidemiological cost and economic cost  following different policies, averaged over $100$ replications. The closer to the left bottom corner, the better. With the shaded areas indicating the 95$\%$ confidence regions.}
\label{figure:Paretosquare}
\end{figure}

\subsection{Sample policies displayed in the demo}
In Figure \ref{fig:pareto_demo}, we apply the policy search algorithm in the threshold-based policy class, and zoom in to analyze three Pareto-optimal policies. 
Here, we give their policy parameters to provide more details. 
For policy A, B, and C, their $\vlam$ is $(0,0)^T$, $(0.26,  420)^T$, and $(245, 573)^T$, respectively. 
This explains their behaviour: policy A is a strict one and assigns level 3 whenever the algorithm believes there is any infectious individual; 
policy B is milder, and it typically imposes the level-2 action unless the spread is quite severe; policy C is much more loose. 


\section{Sensitivity analysis}\label{sec: supp-robust}

\subsection{Robustness against model missepcification}\label{sec: supp-robust-analysis}
In this section, we investigate the robustness of the proposed framework against potential model missepcification. 
We use a generalized Susceptible-Exposed-Infected-Removal model (SEIR) model instead of the GSIR model as the data generation model, and conduct a simulation study similar with the one in Section \ref{sec:numerical_policy}. 
% with the setting kept the same
The standard SEIR model is another commonly used compartmental model, which adds one additional exposed compartment to the SIR model. 
See Figure \ref{figure:SEIR} for an illustration and refer to \cite{tang2020review} for a detailed introduction. 

\begin{figure}[h!]
\centering
\includegraphics[width=.5\textwidth]{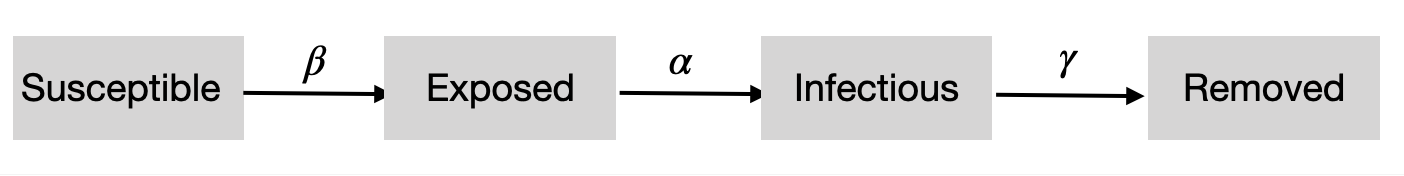} 
\caption{A diagram for the standard SEIR model.}
\label{figure:SEIR}
\end{figure}

We generalize the SEIR model in a similar with as the GSIR model, by including the action effects into consideration to set the infection rate $\beta$. The transition from the susceptible compartment to the exposed compartment is assumed to follow a binomial distribution with parameter $\alpha$. 
According to \cite{yang2020modified}, we set the incubation rate $\alpha$ as $1/7$. 
The other parameters are kept the same with Section \ref{sec:numerical_policy}. 
Since the exposed compartment is typically latent,  the number of individuals in this compartments on the beginning date can not be set based on the real data as the other compartments. 
For experiment purpose, we set the number to be the same with the number in the infectious compartment. 

The results are presented in Figure \ref{figure:Pareto_SEIR}. 
As expected, compared with results under the GSIR model, the performance of the  proposed method under this setting slightly deteriorates. 
However, in generally, the method still over-performs the other fixed policies, and also provides more options with a clear trade-off.  



\begin{figure}[h!]
\centering
\includegraphics[width=.5\textwidth]{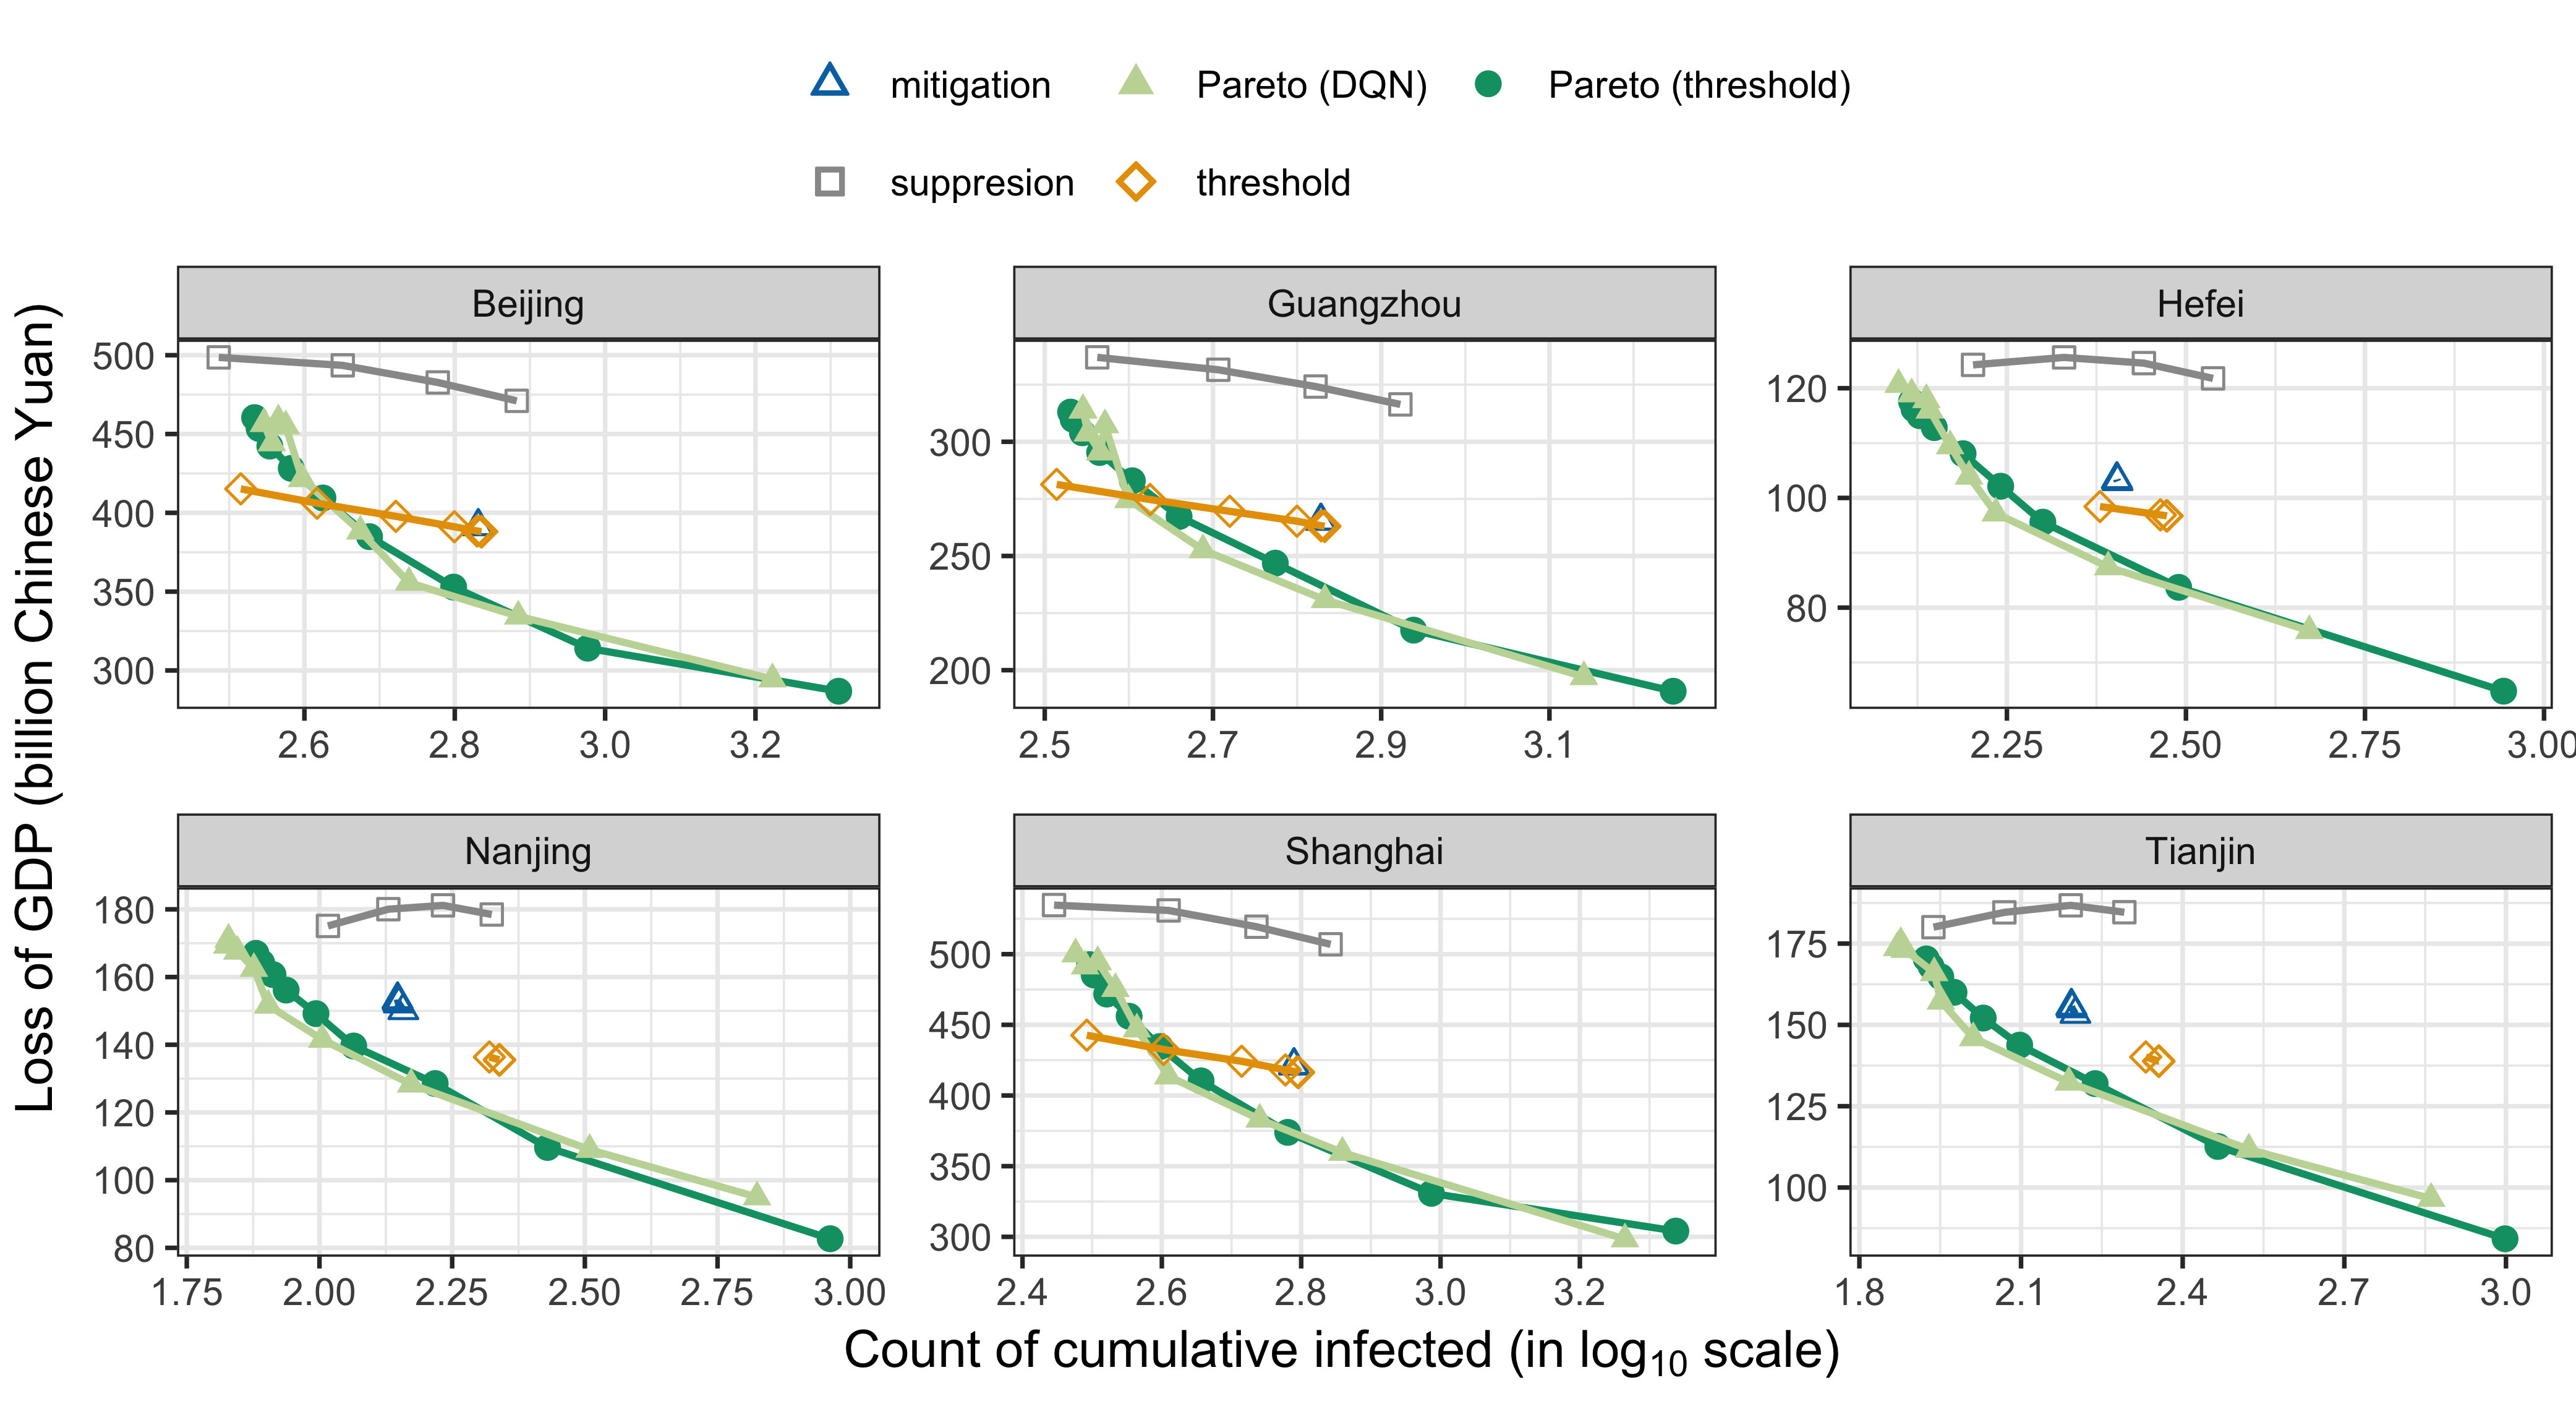} 
\caption{Simulated results when the true data generation model is the generalized SEIR model. Cumulative epidemiological cost and economic cost  following different policies, averaged over $100$ replications.}
\label{figure:Pareto_SEIR}
\end{figure}


\subsection{Hyper-parameter sensitivity analysis}\label{sec:sensitivity}
Our framework requires selecting several hyper-parameters according to domain knowledge, and our choices in the experiments largely follow the practice in the early period of the COVID-19 outbreak and are listed in Section \ref{sec:supp-data}. 
On one hand, at the beginning of an pandemic we have to rely on some priors to make decision; and on the other hand, in this section we use numerical experiments to evaluate the robustness of our algorithm to these hyper-parameters. 
The setting is kept the same with Section \ref{sec:numerical_policy}, except for that we only run 25 replications for the proposed algorithm to save computation. 
We present results for the threshold-based policy class. 
Results for the DQN-based methods are similar and omitted. 

In Figure \ref{figure:robust_lag}, we report the results with $D = 7, 8, 9, 10, 11$. 
It can be seen that, although the results varies a little, the algorithm generally still outperform the competing policies, and our findings in Section \ref{sec:numerical_policy} still hold. 

% \begin{figure}[h!]
% \centering
% \includegraphics[width=.45\textwidth]{figures/robust_lag.png} 
% \caption{Robust analysis results for the hyper-parameter $D$.}
% \label{figure:robust_lag}
% \end{figure}

% \begin{figure}[h!]
% \centering
% \includegraphics[width=.45\textwidth]{figures/robust_effect.png} 
% \caption{Robust analysis results for the hyper-parameter $\mu_1$ and $\mu_2$.}
% \label{figure:robust_effect}
% \end{figure}


\begin{figure*}[t]
\begin{subfigure}{.45\textwidth}
\centering
\includegraphics[width=.8\textwidth]{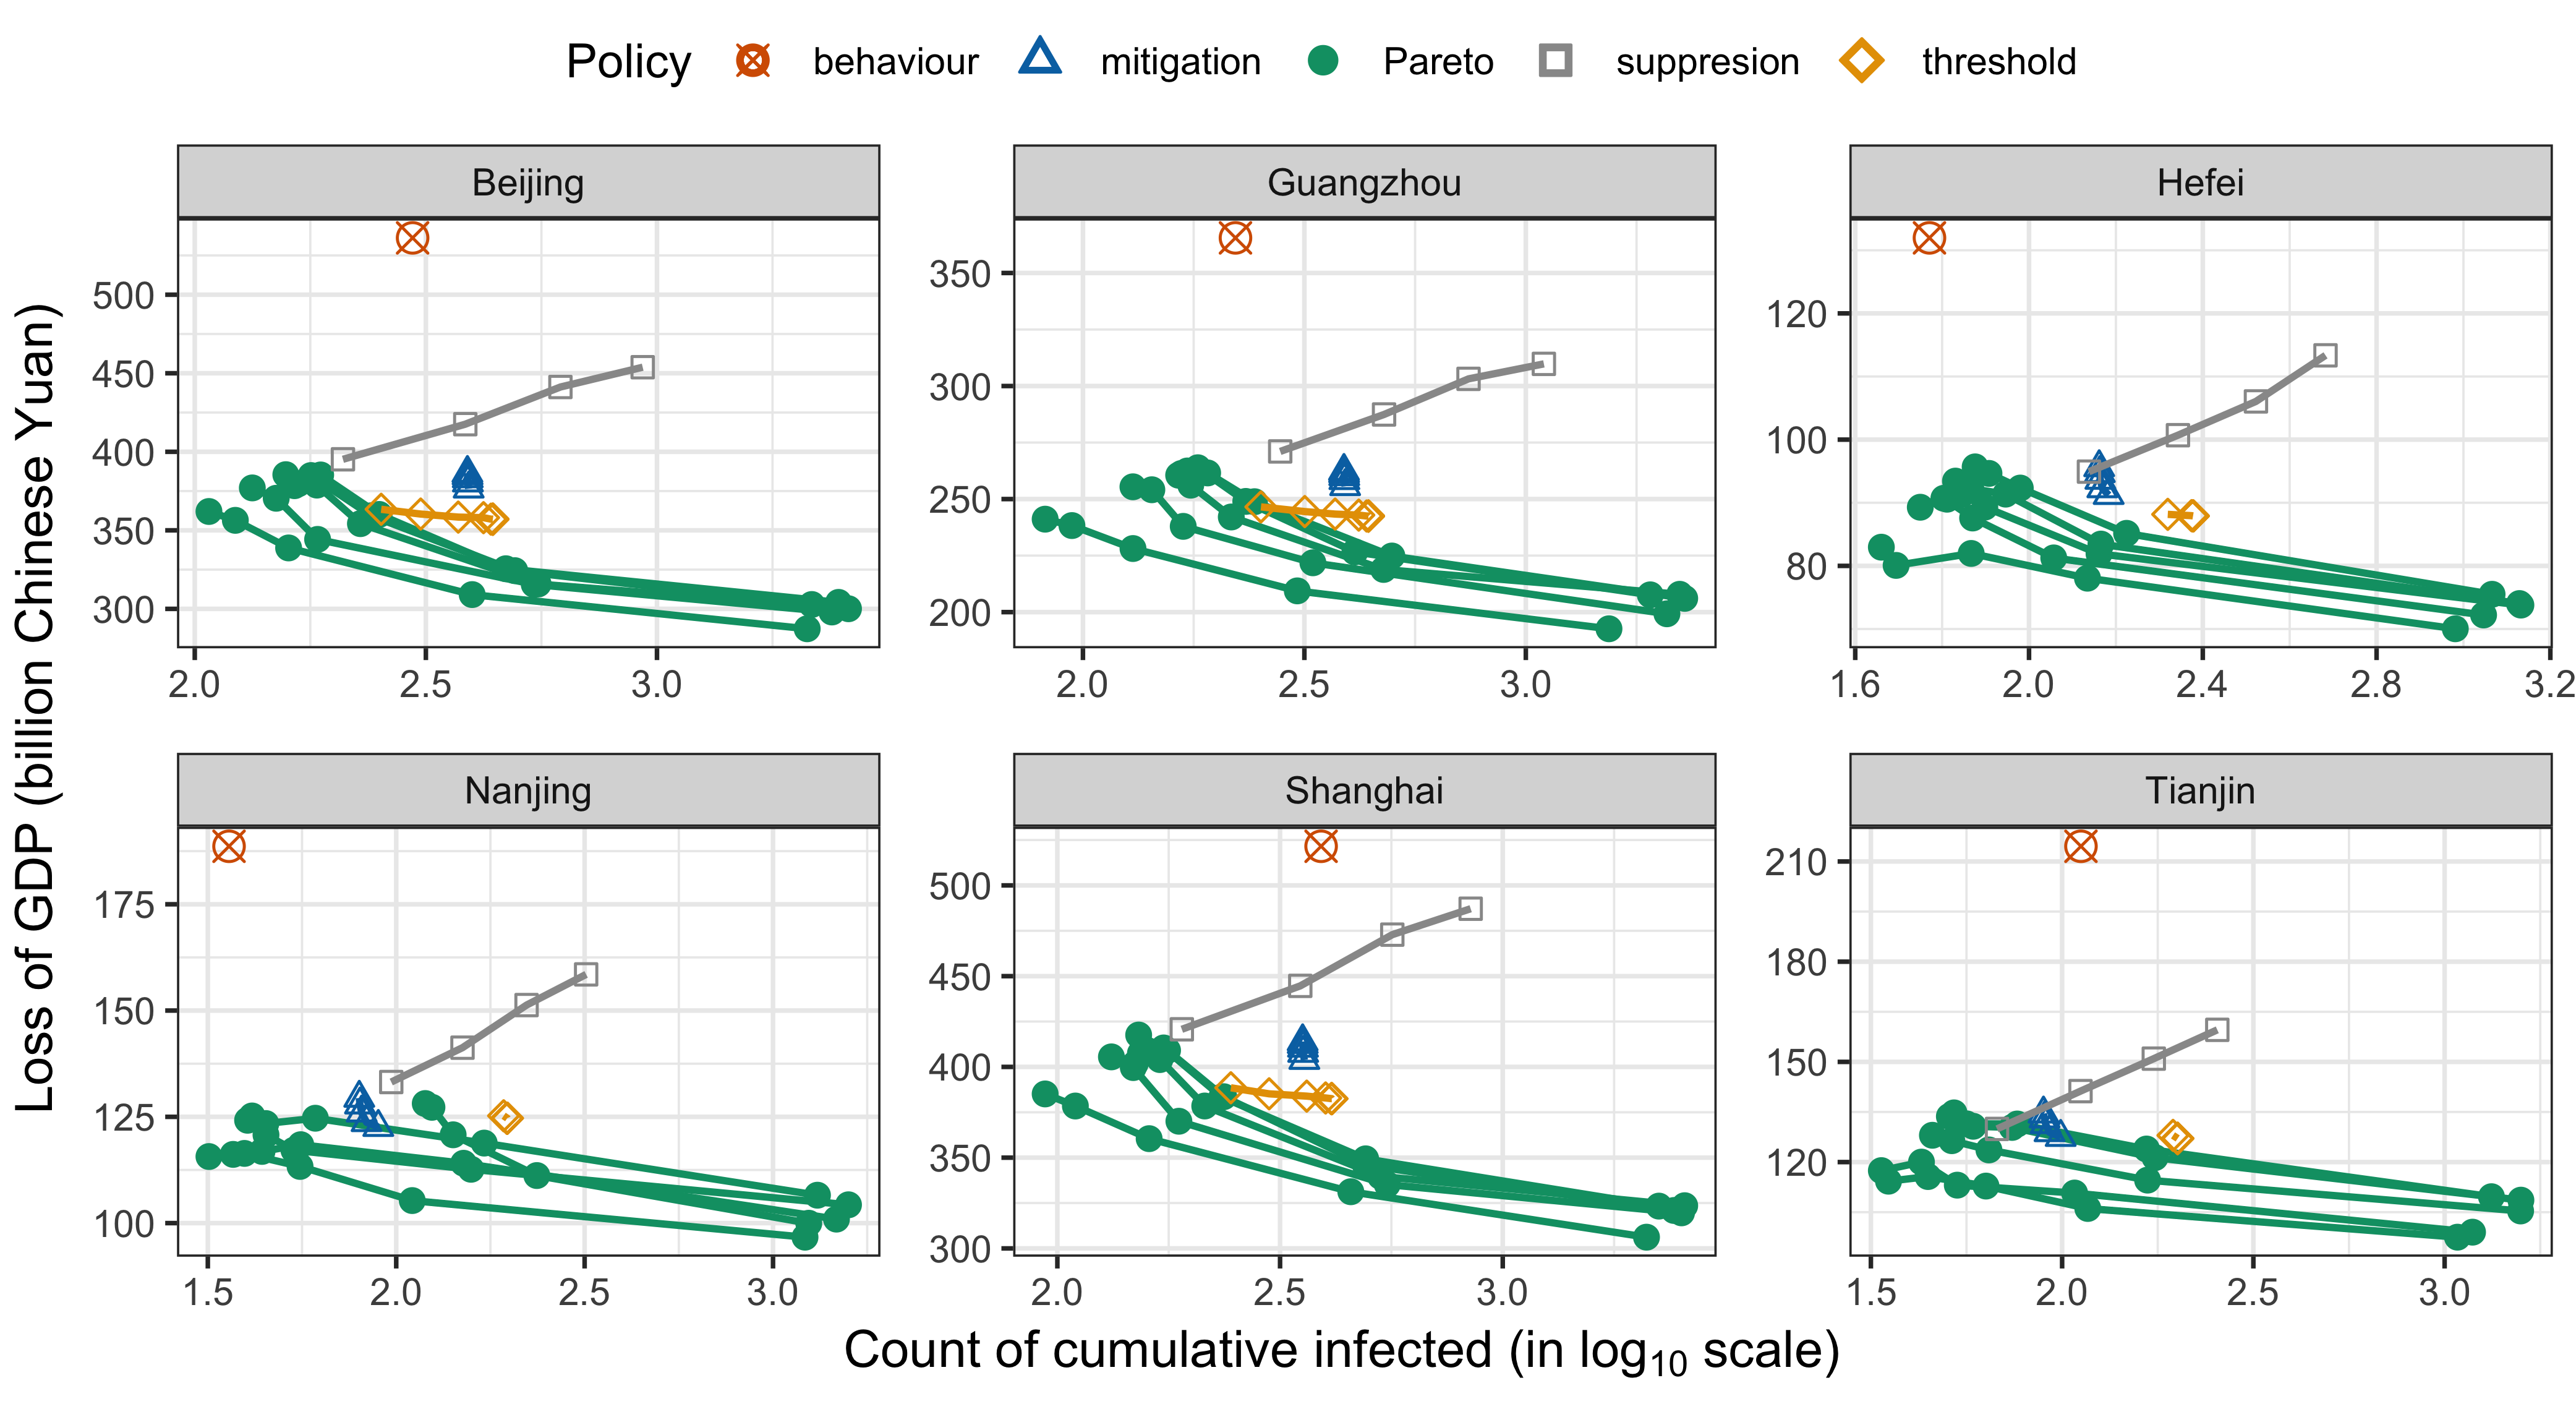} 
\caption{Robust analysis results for the hyper-parameter $D$.}
\label{figure:robust_lag}
\end{subfigure}
\begin{subfigure}{.45\textwidth}
\centering
\includegraphics[width=.8\textwidth]{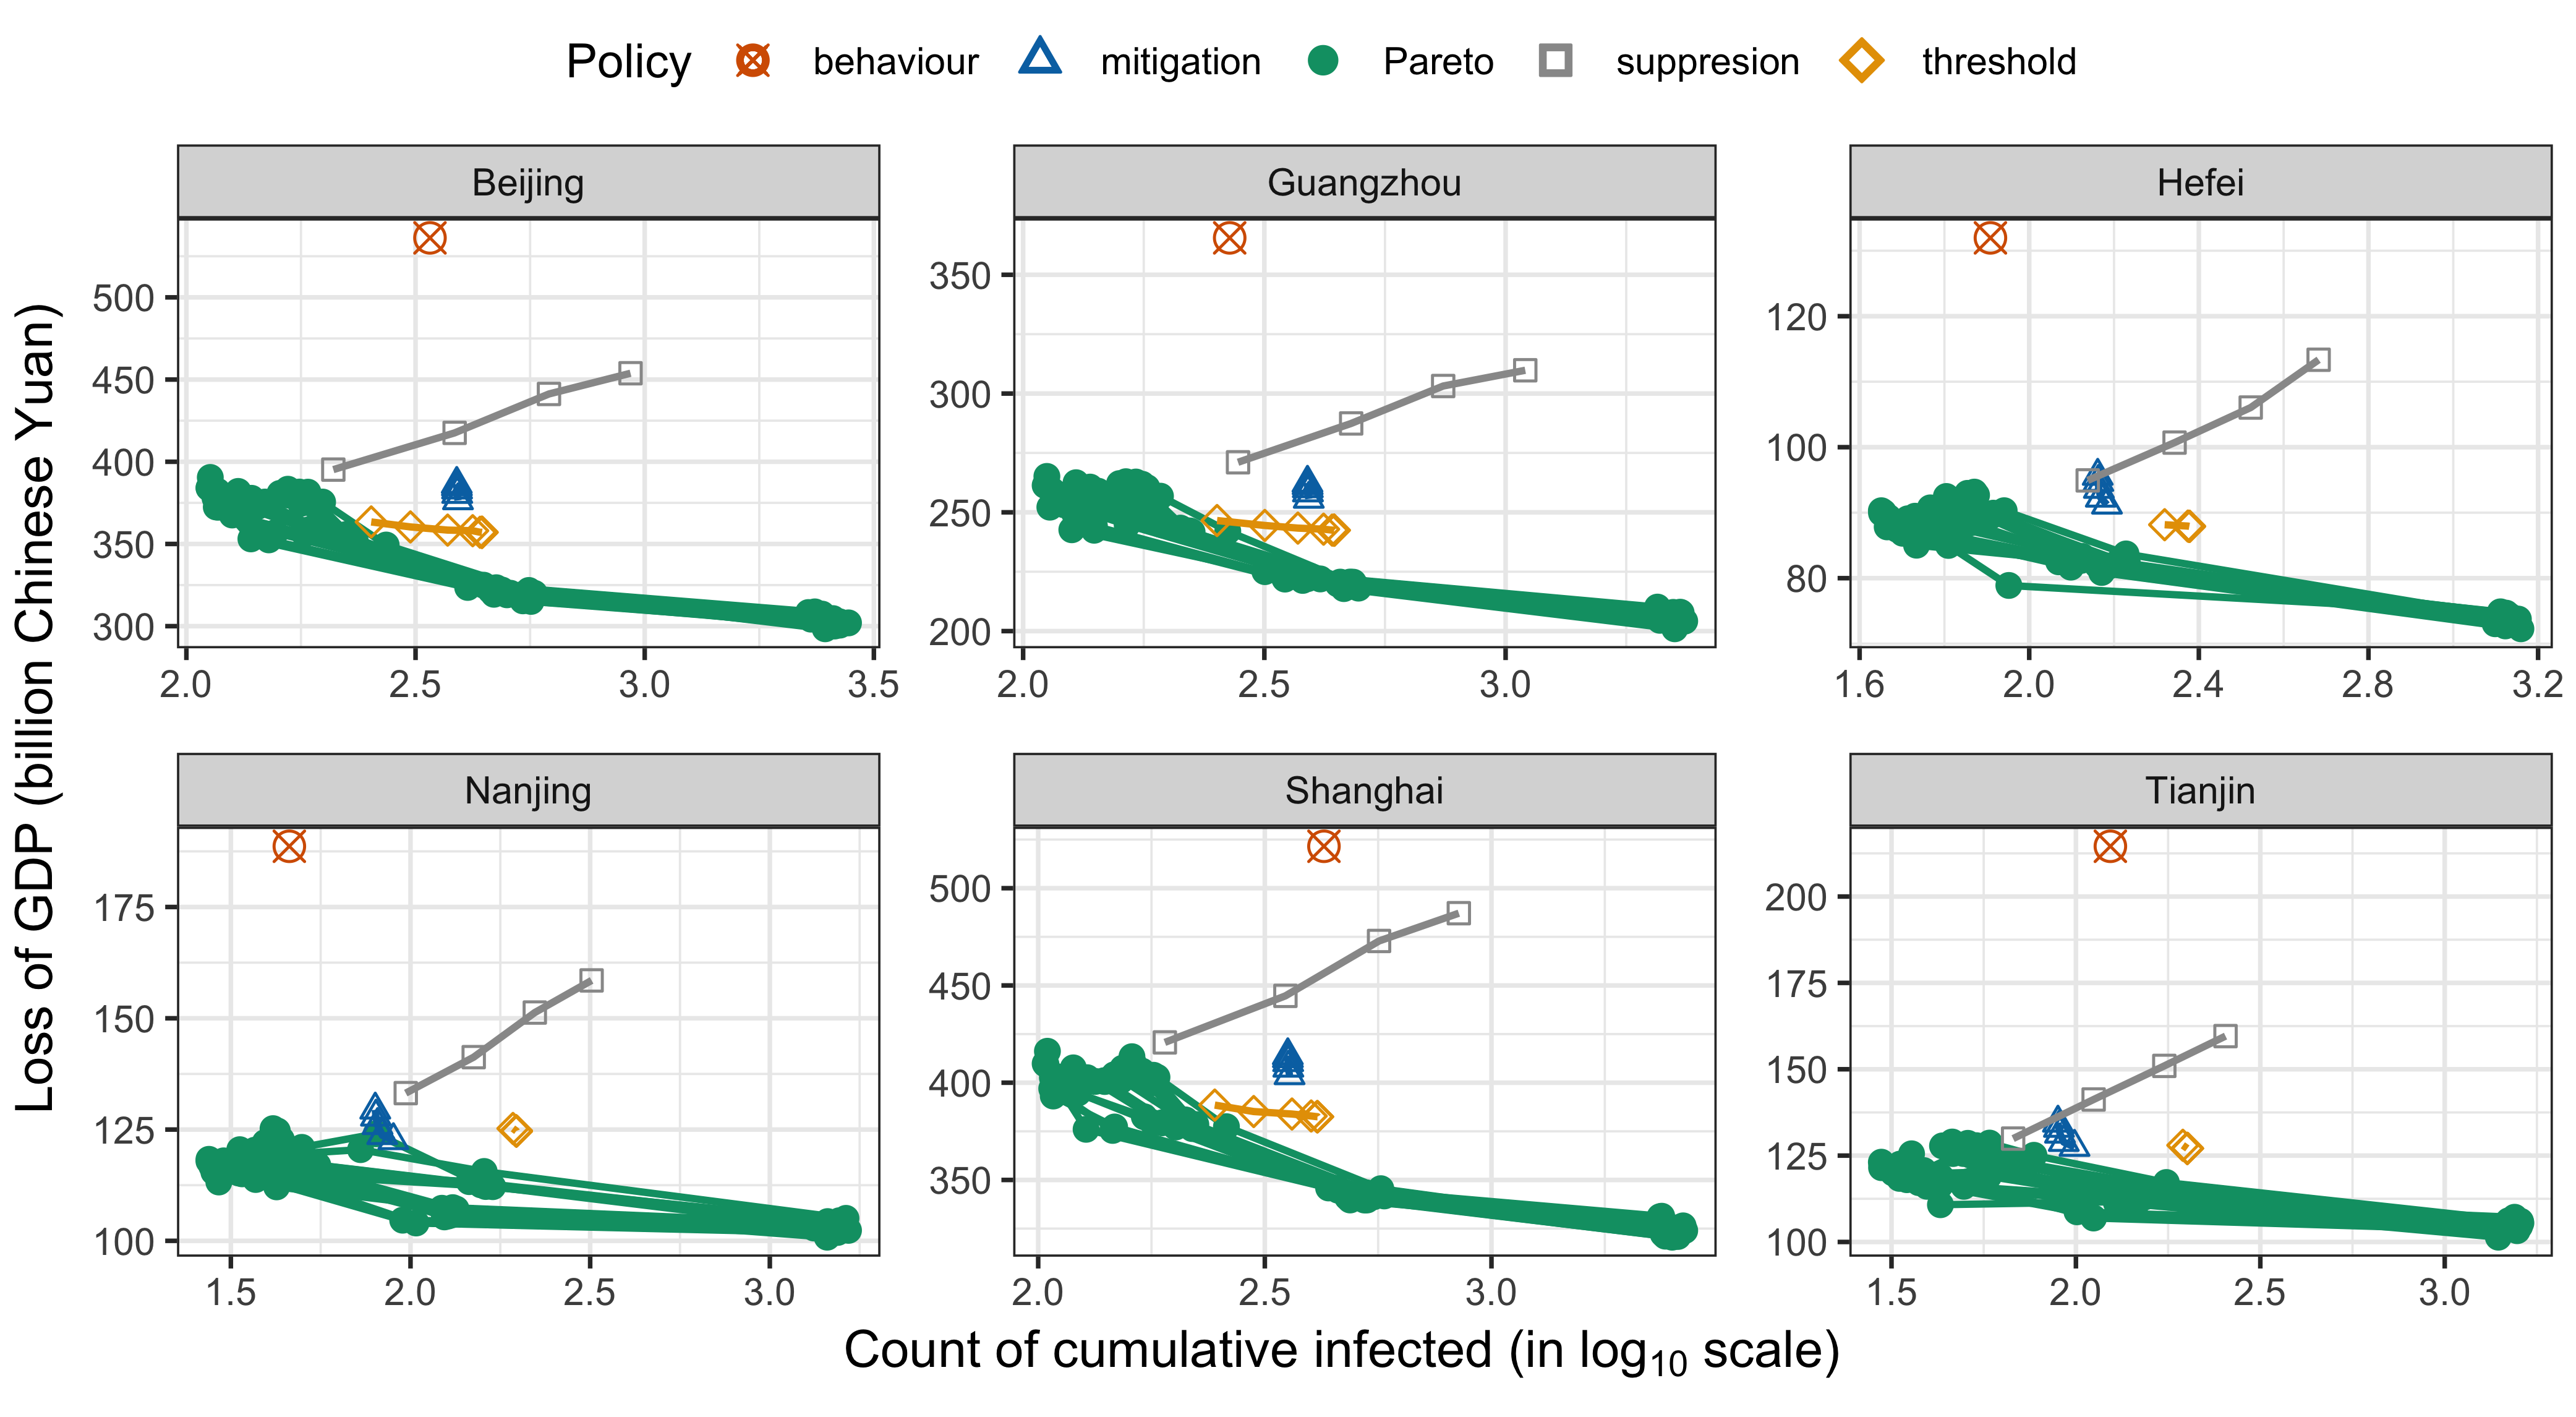} 
\caption{Robust analysis results for the hyper-parameter $\mu_1$ and $\mu_2$.}
\label{figure:robust_effect}
\end{subfigure}
\caption{Hyper-parameter sensitivity analysis}
\label{fig:sensitivity}
\end{figure*}



Similarly, we report the robustness analysis results for the treatment effects $\mu_2$ and $\mu_3$ In Figure \ref{figure:robust_effect}. 
Recall that we define $\mu_j = \beta_j / \beta_1$ and use it to set the prior for $\beta_i$. 
In our experiment, we use $\mu_2 = 0.2$ and $\mu_3 = 0.1$. 
In this analysis, we present results for $\{(\mu_2, \mu_3): \mu_3 \in \{0.05, 0.1, 0.15, 0.2\}
, \mu_2 - \mu_3 \in \{0.05, 0.1, 0.15, 0.2\} )\}$. 
These prior parameters turn out have little important in the long run, because their effects get washed out quickly by the observed data. 
The findings for the other prior parameters are similar. 

\break

\bibliography{bib}
\bibliographystyle{plain}
	
\end{document}
